# Supplementary material for: PointGMM: a Neural GMM Network for Point Clouds
Source: arXiv:2003.13326 ancillary file (2020-03-30)
Supplement: Supplementary file 1 [file supplementary_material.pdf]

## PointGMM: a Neural GMM Network for Point Clouds

# Supplementary Material

This document contains additional qualitative results to the paper *PointGMM: a Neural GMM Network for Point Clouds*, demonstrating the capabilities of PointGMM as a generative model.

**Pages 2 — 7** contain additional, enlarged sampled shapes. To highlight correspondence between different parts in different shapes, below each shape, we isolate points that were sampled from the same group of Gaussians at the first level of their hGMM tree. Notice that in all shapes, the same group of GMMs consistently correspond to the same spatial location in the shape.

**Pages 8 — 10** contain additional latent space interpolation examples.

**Page 11** contain quantitative comparison to other point clouds generative methods.

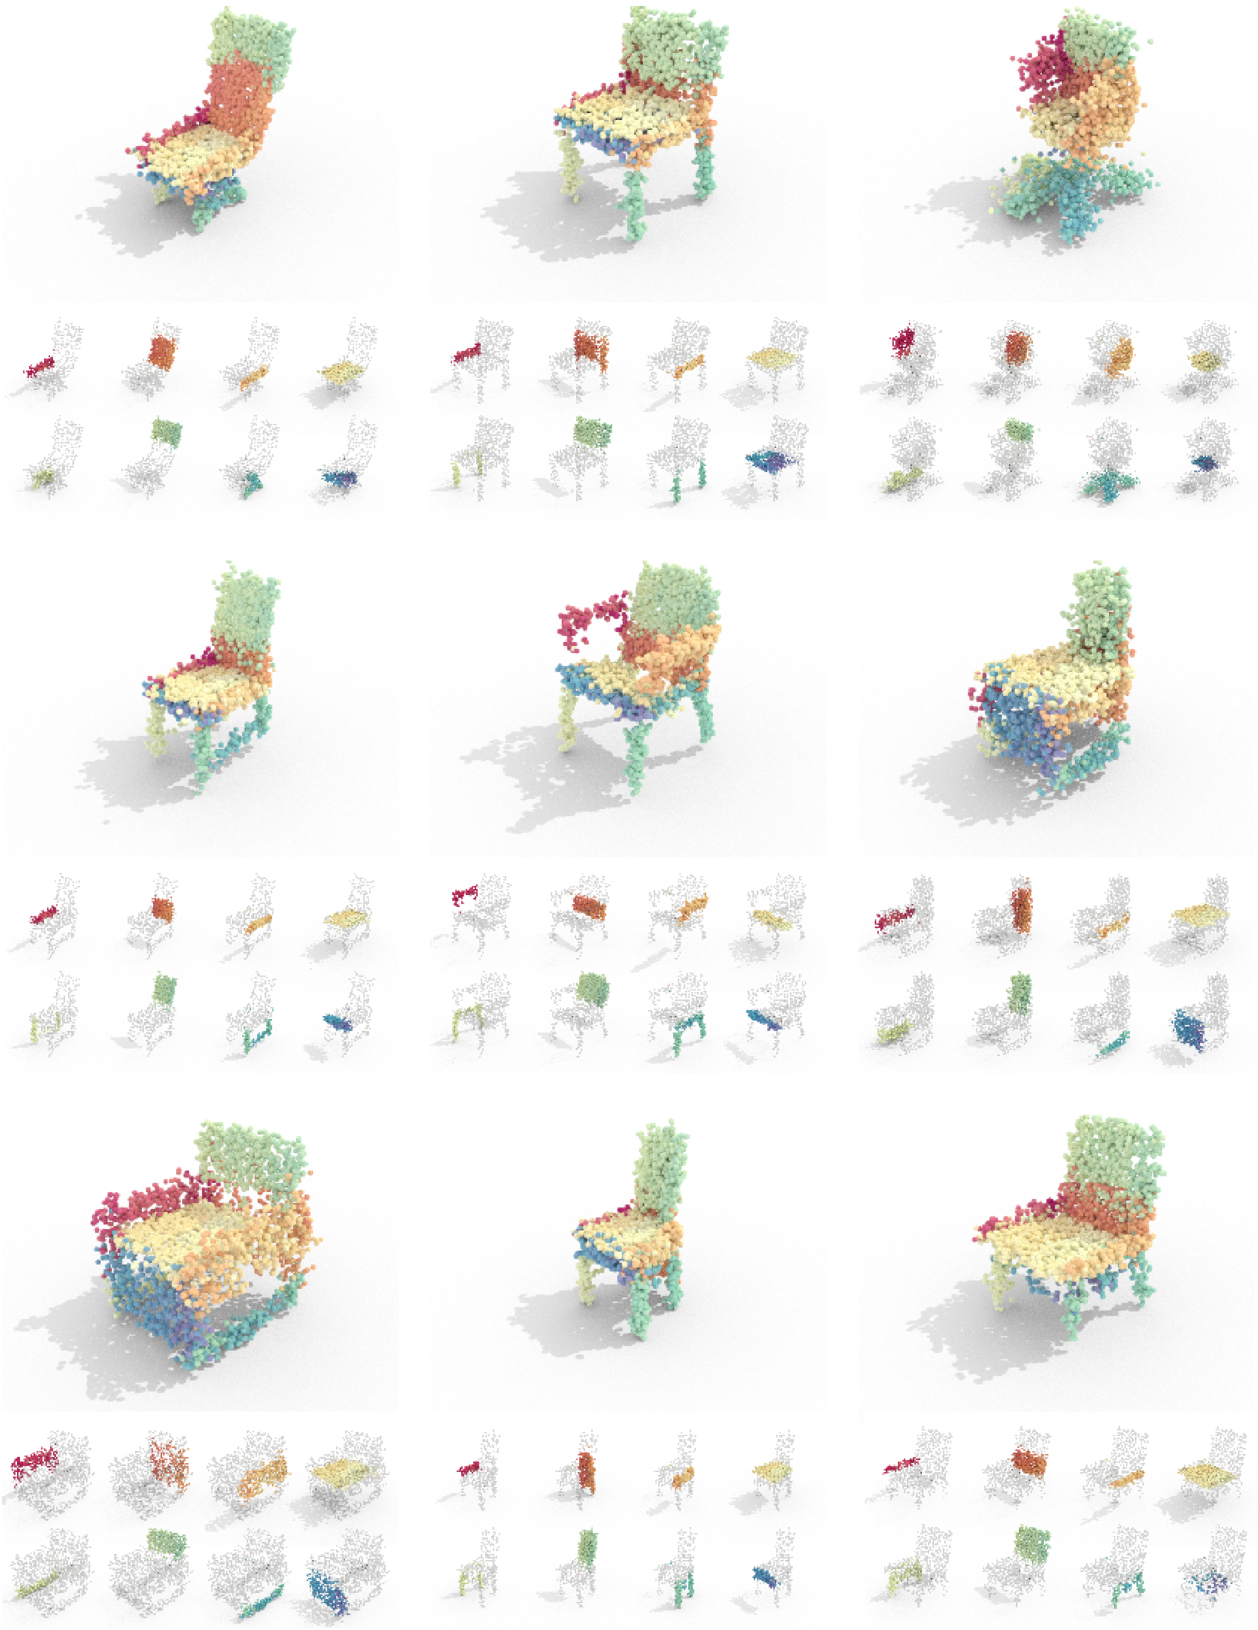

Figure 1: Sampled chairs

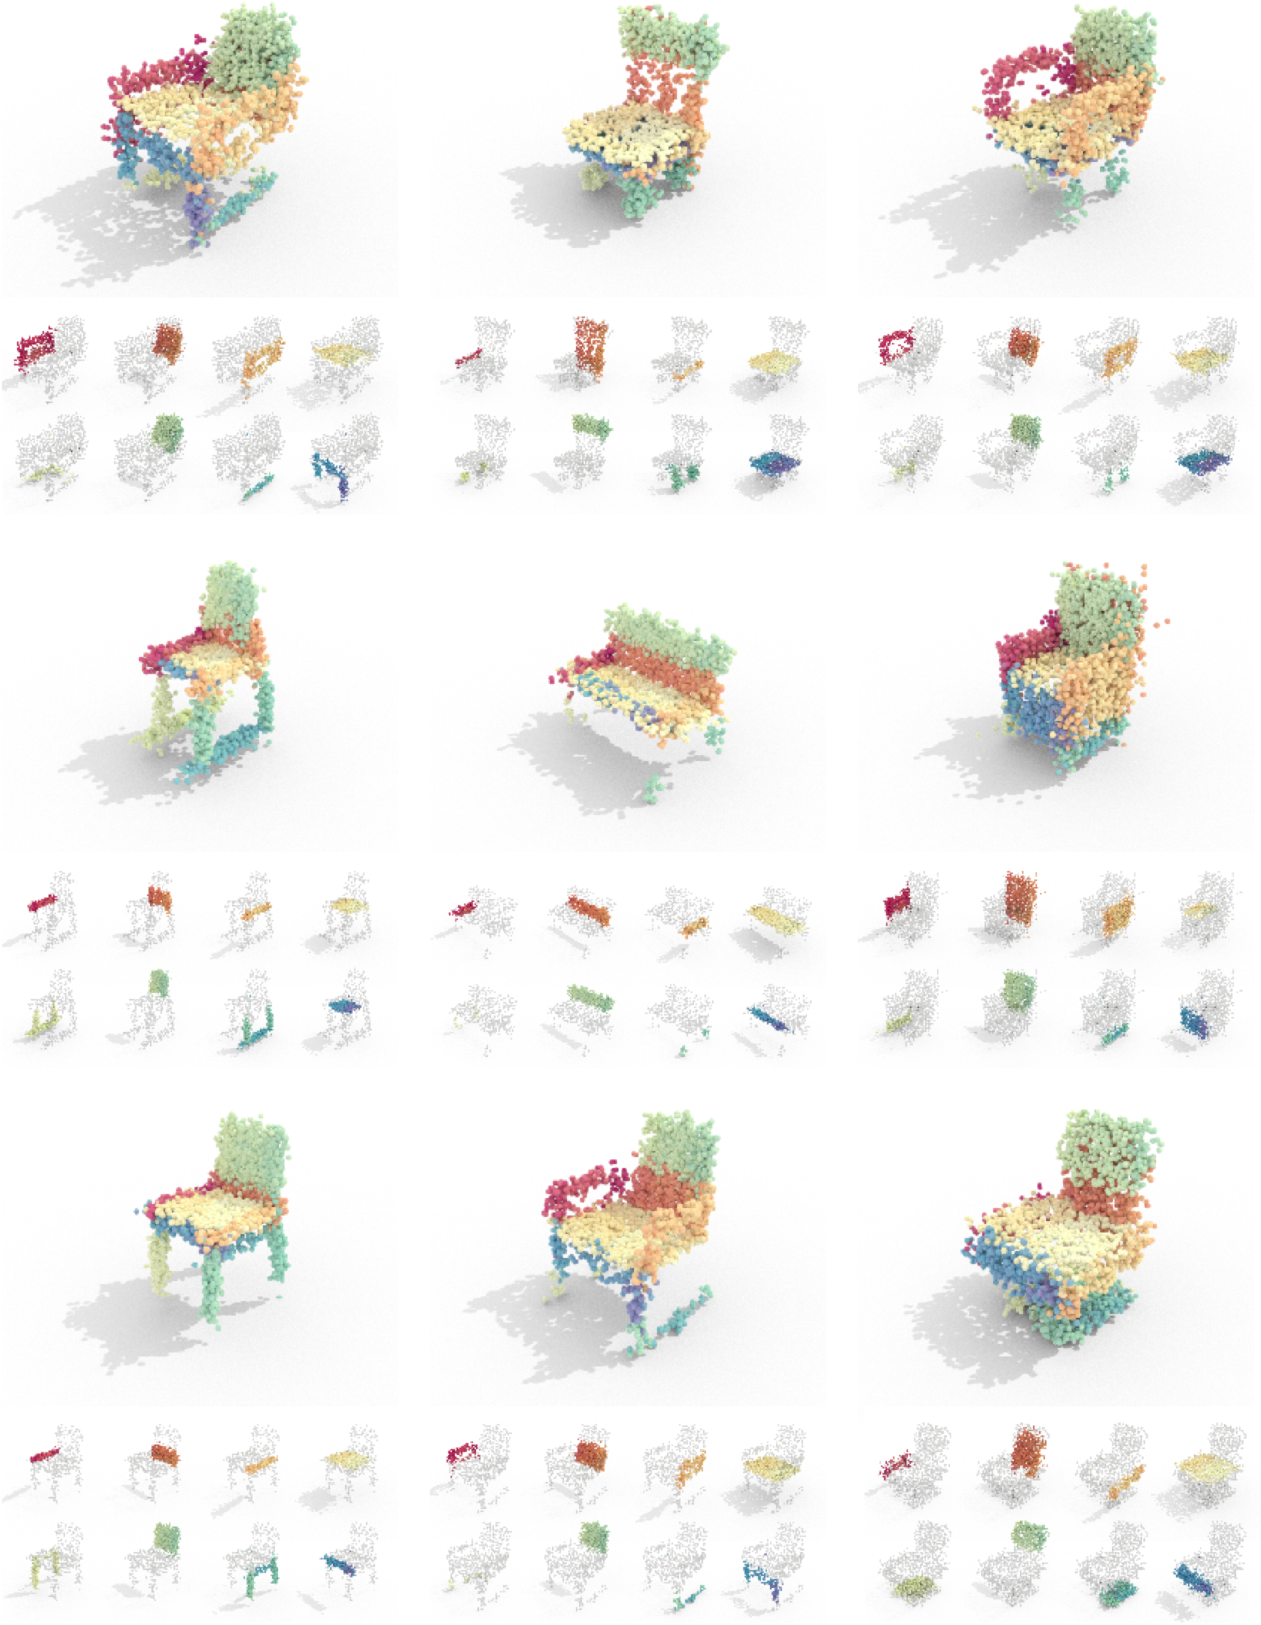

Figure 2: Sampled chairs

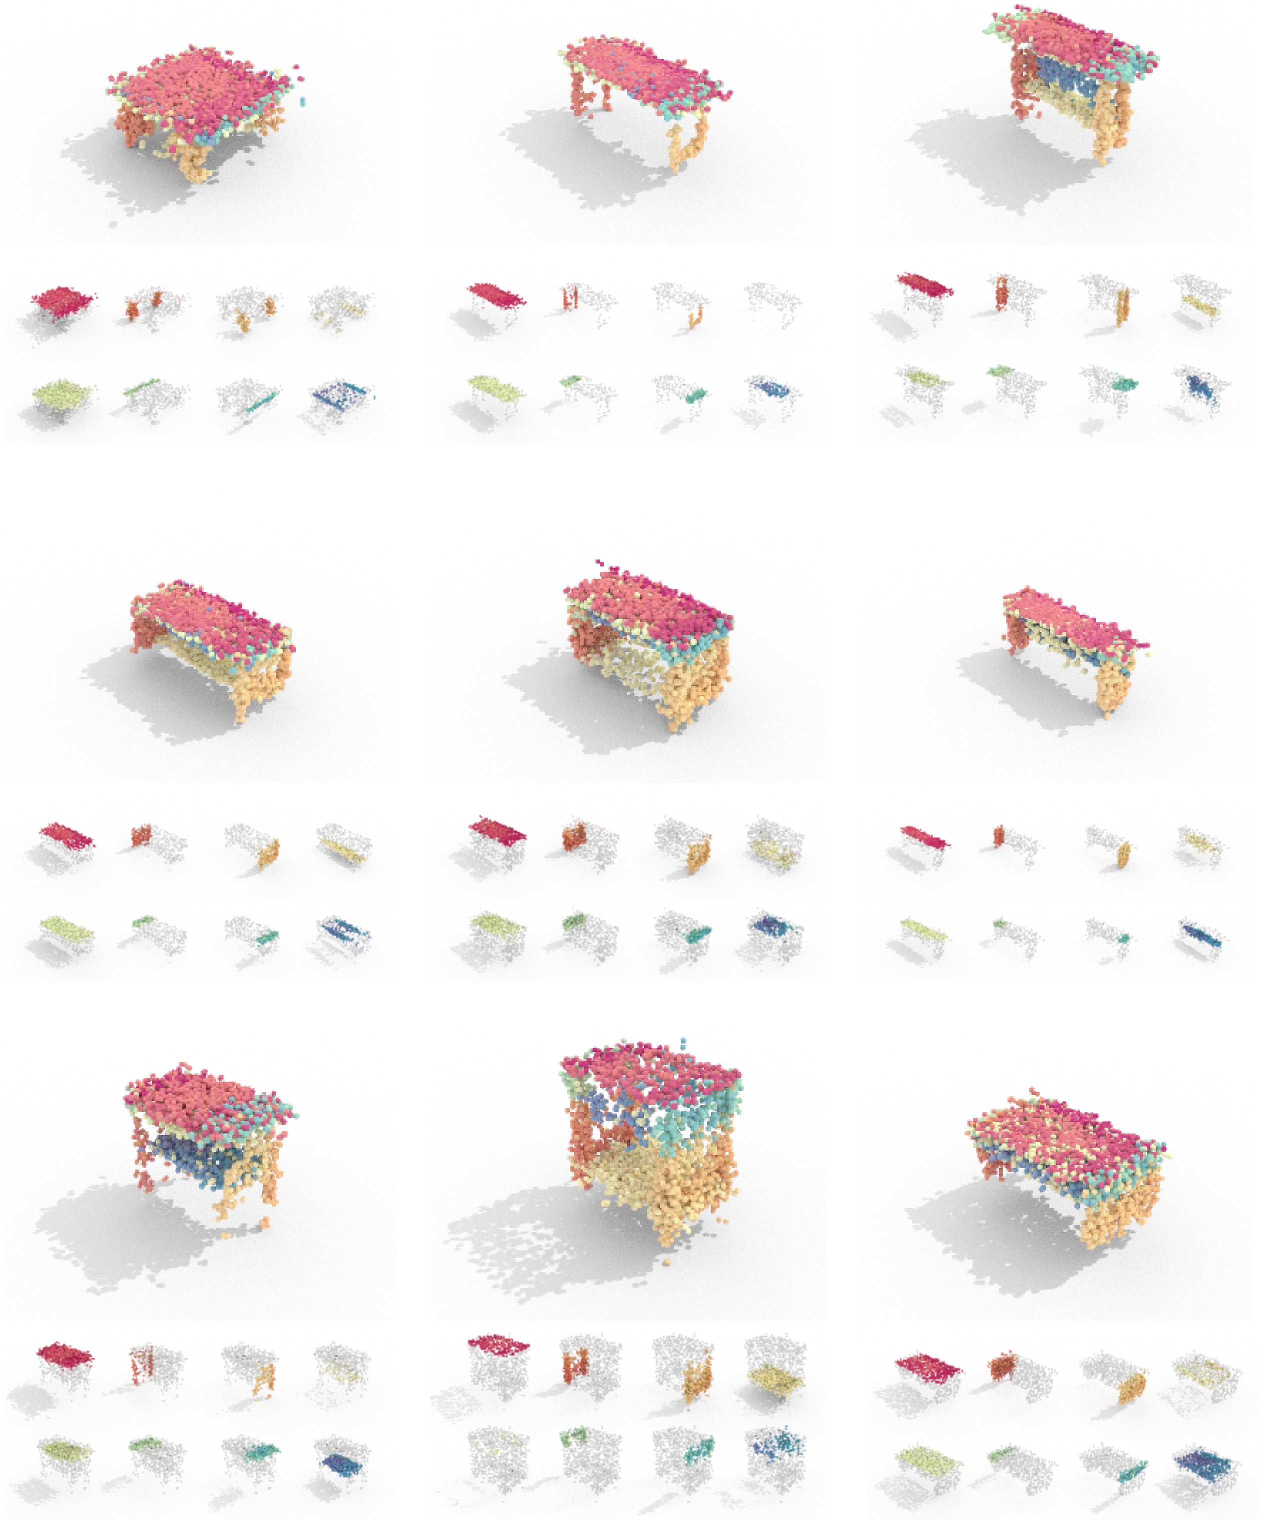

Figure 3: Sampled tables

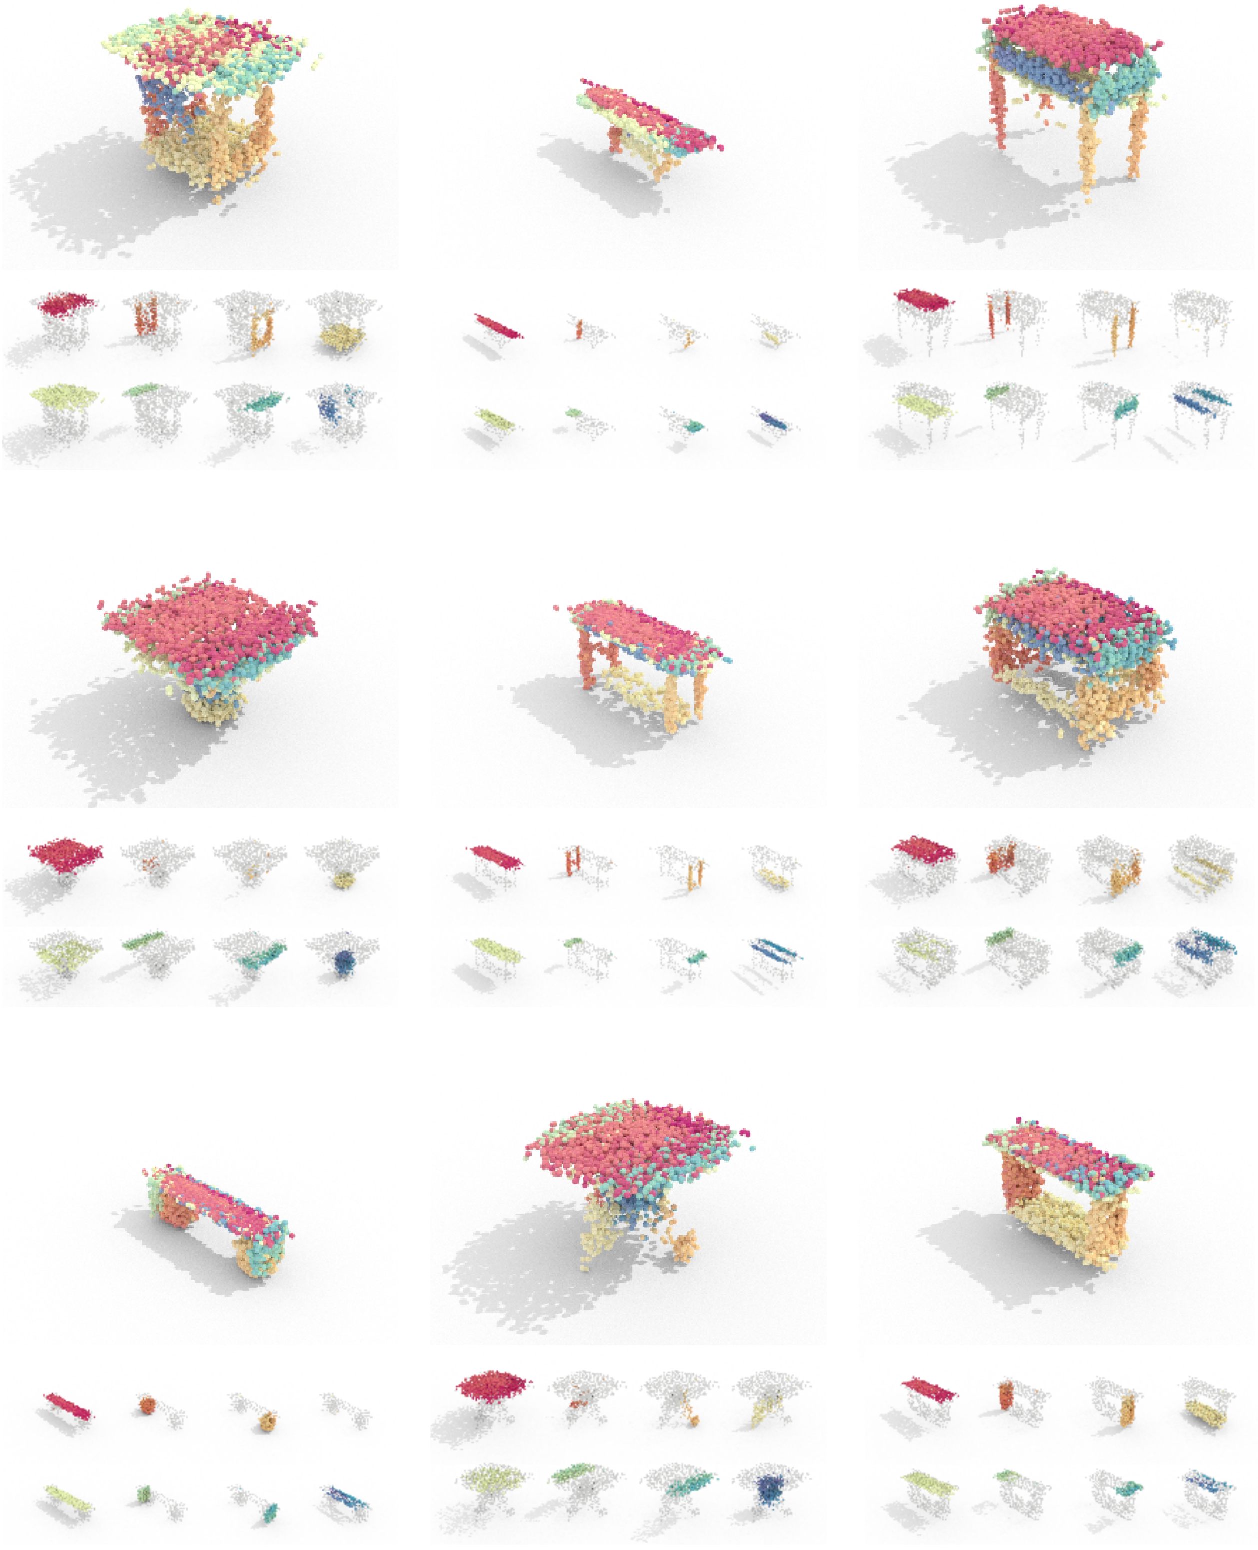

Figure 4: Sampled tables

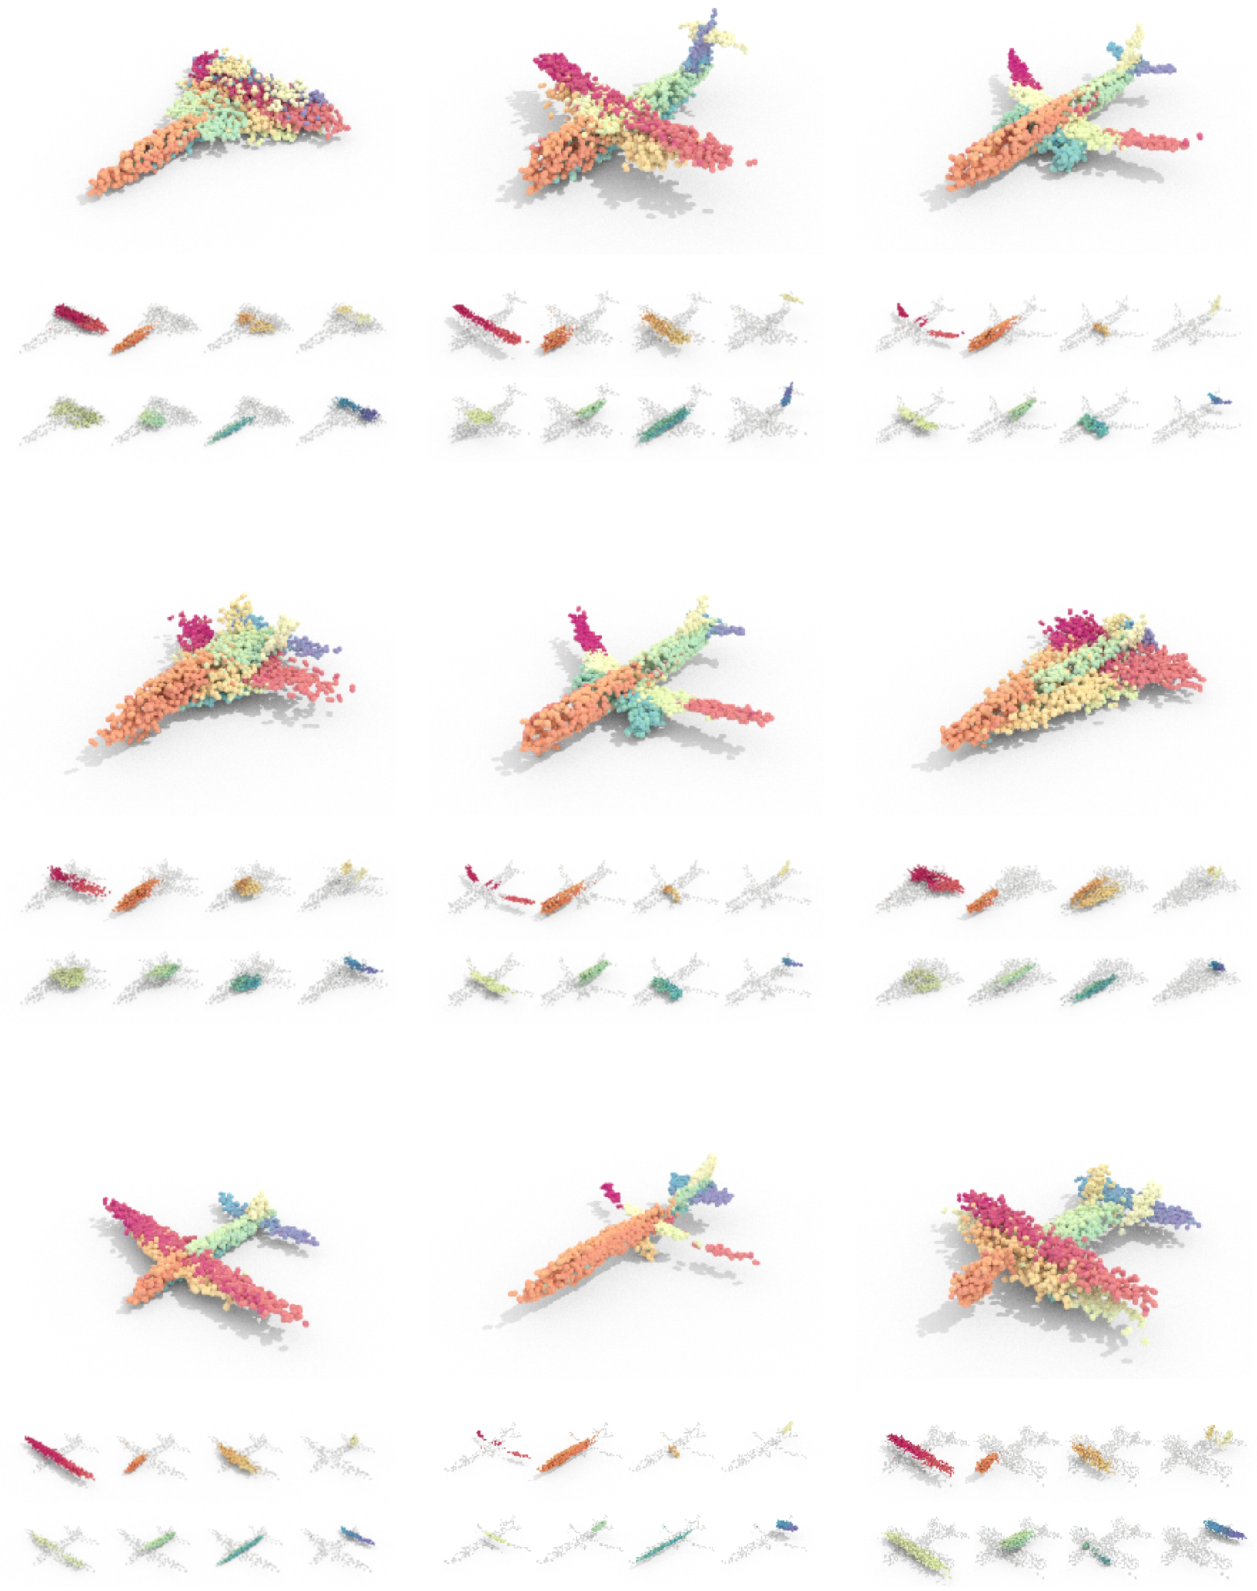

Figure 5: Sampled airplanes

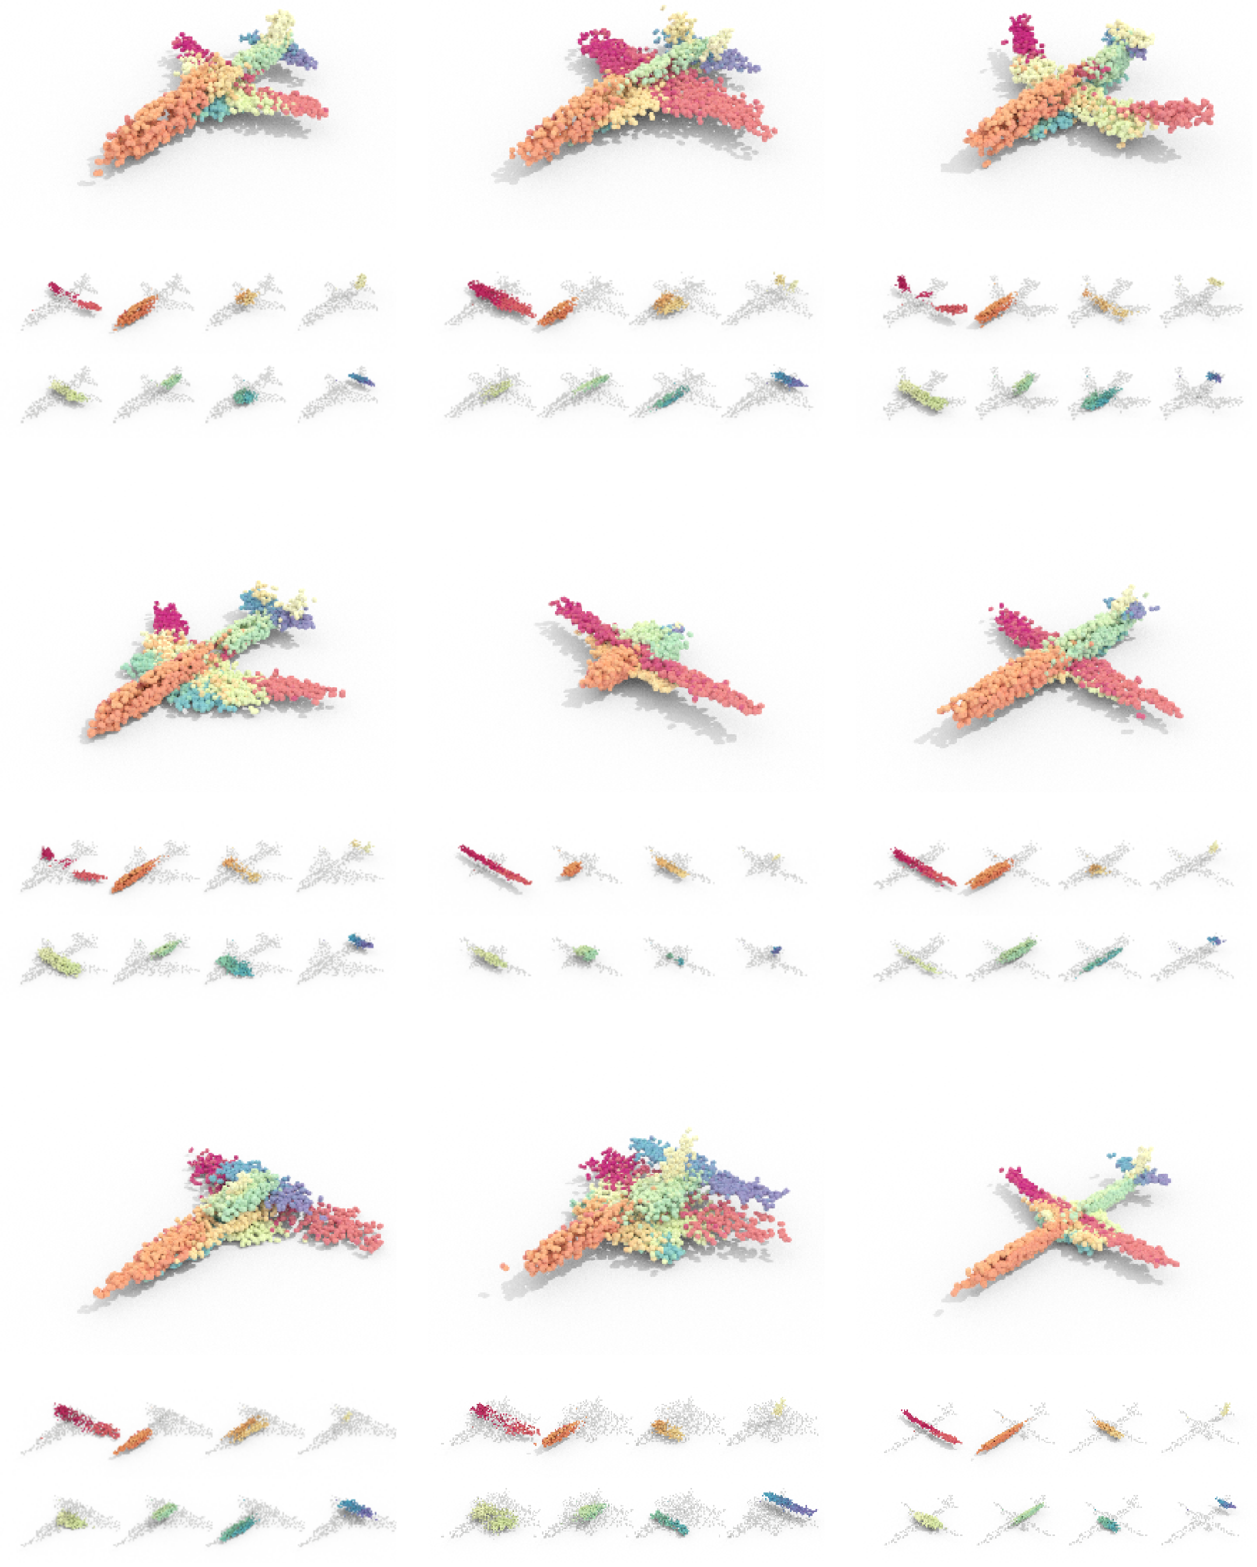

Figure 6: Sampled airplanes

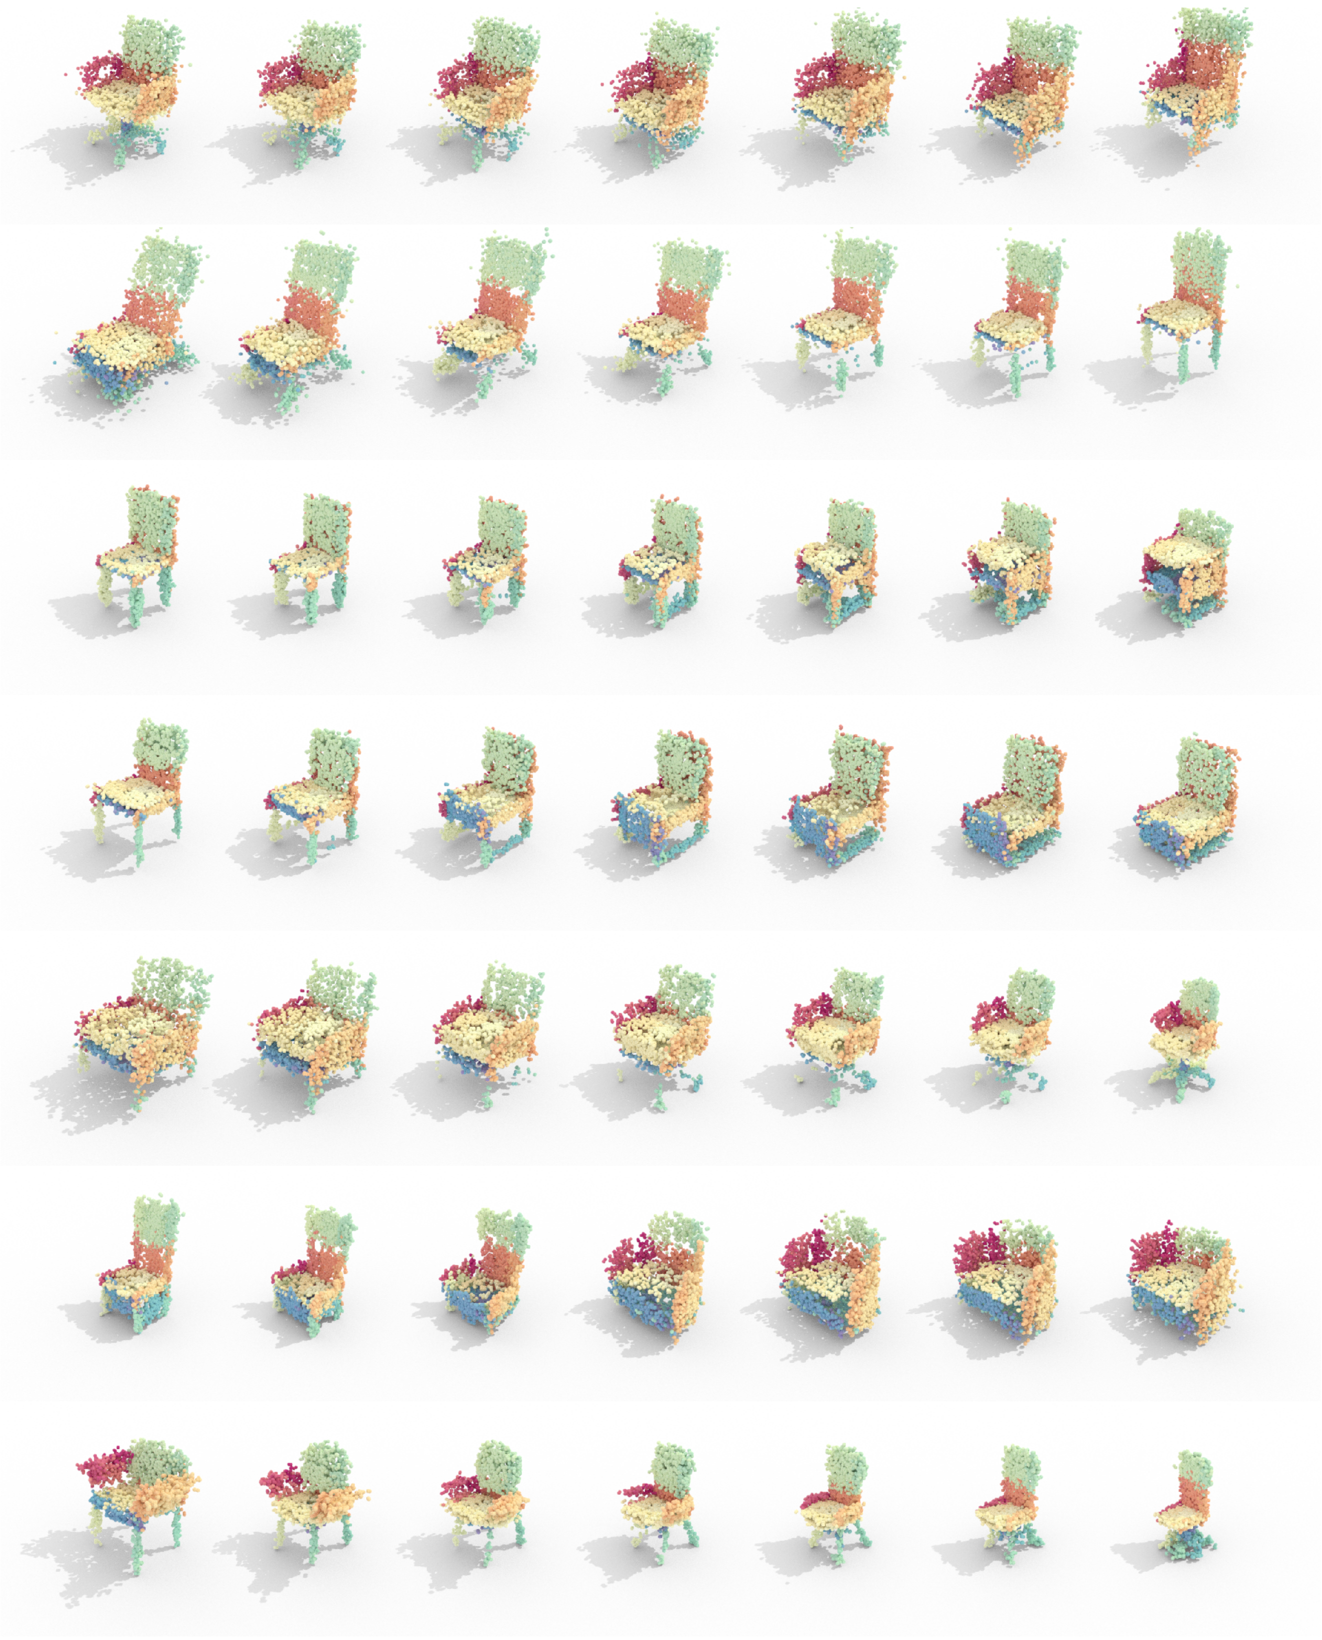

Figure 7: Chairs interpolations.

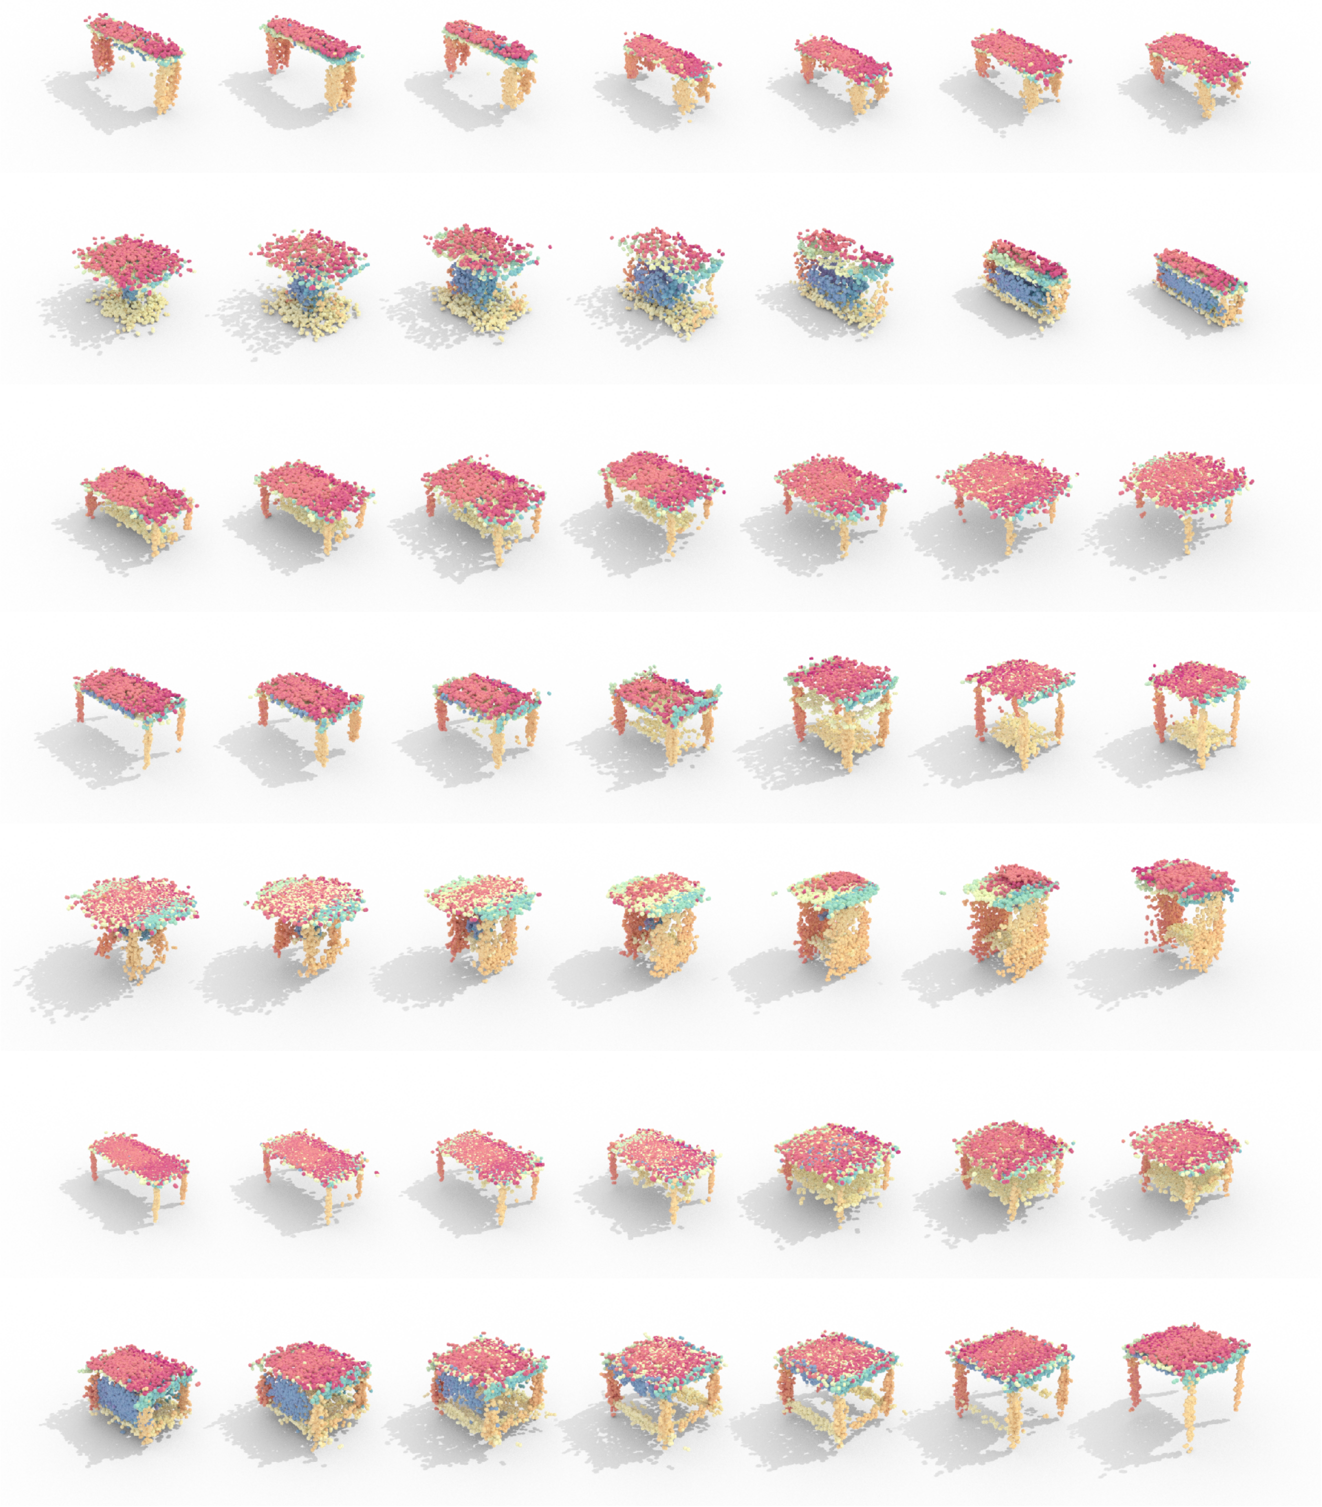

Figure 8: Tables interpolations.

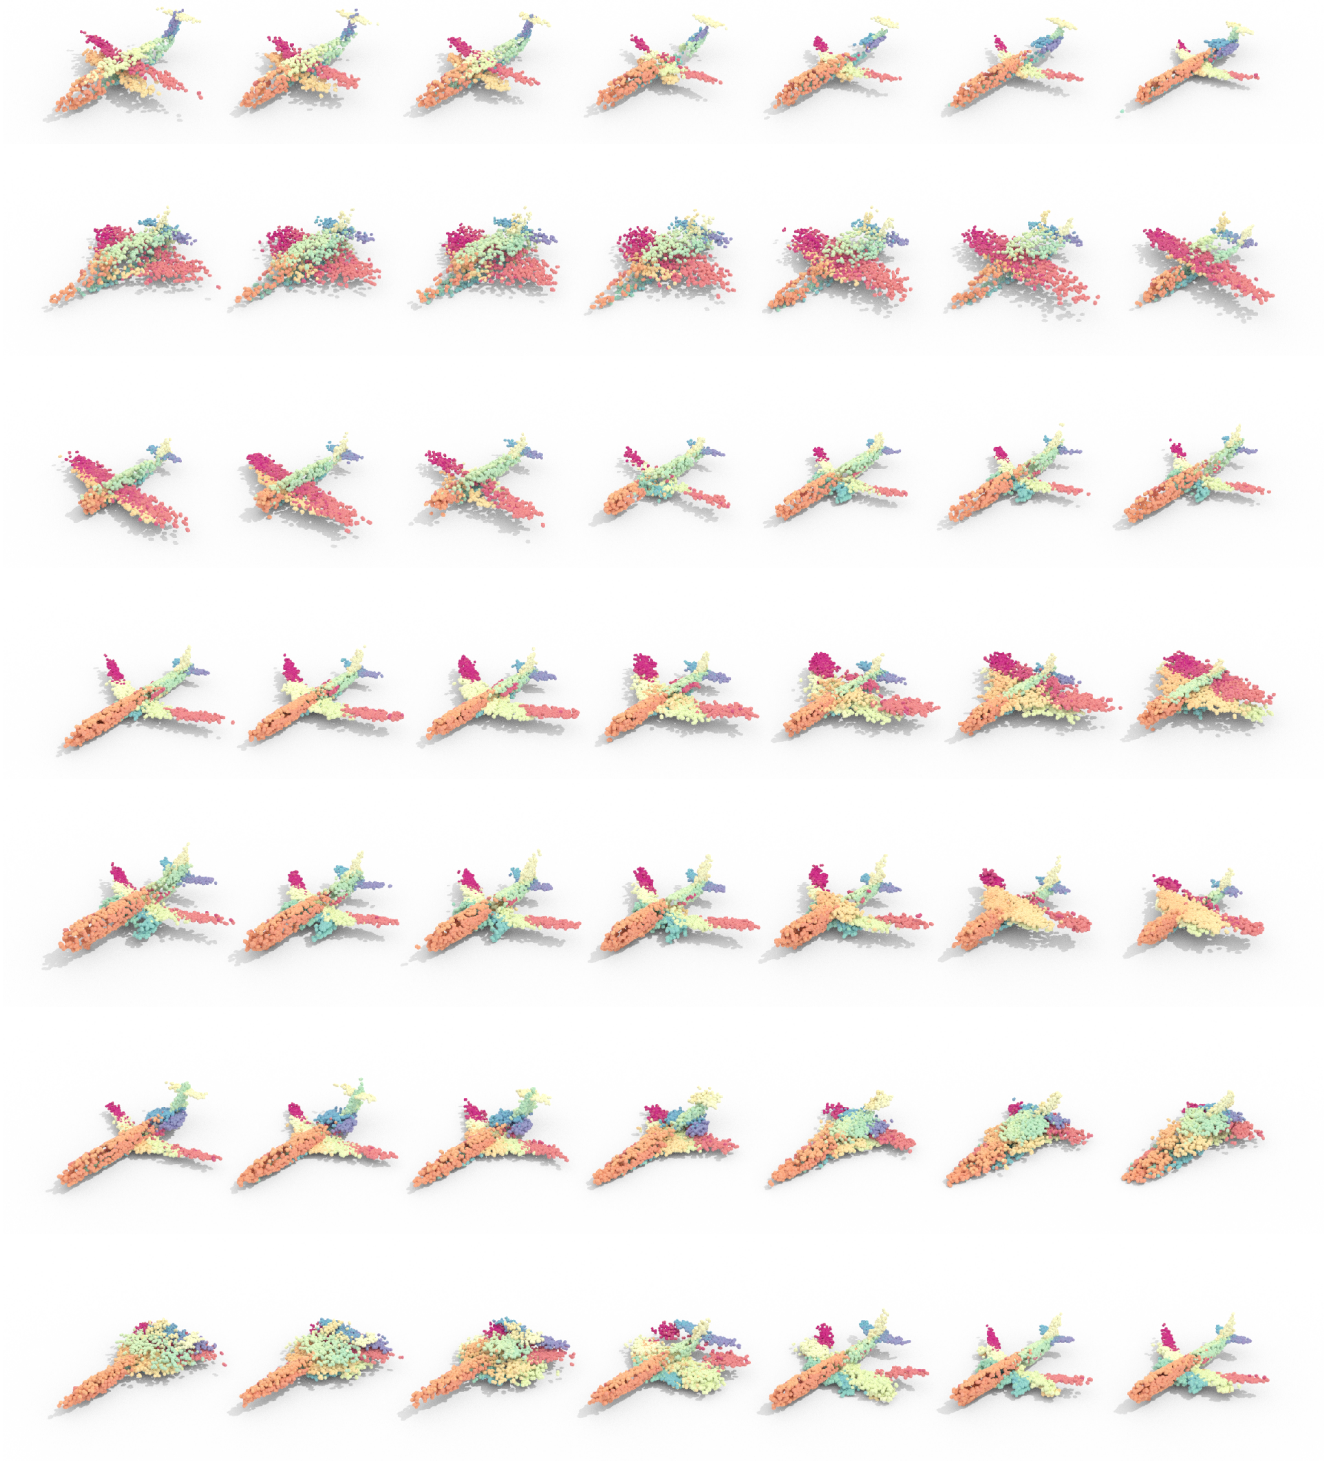

Figure 9: Airplanes interpolations.

**Quantitative results.** We evaluate our generative approach using the same metrics as Yang *et al.* [2] which includes Jensen-Shannon Divergence (JSD), Minimum matching distance (MMD), Coverage (COV) and 1-nearest neighbor accuracy (1-NNA). We train and test our method using the same data partitions and categories and add our results to the their comparison table 1. The other generative approaches we compared too are raw-GAN [1], latent-GAN [1], PC-GAN [3] and PointFlow. [2]. The full details about the evaluation metrics and the comparison test, may be found in [2].

| shape | Model | JSD (↓) | MMD (↓) | | COV (% ↑) | | 1-NNA (% ↑) | |
|---|---|---|---|---|---|---|---|---|
| | | | CD | EMD | CD | EMD | CD | EMD |
| chair | r-GAN | 11.5 | 2.57 | 12.8 | 33.99 | 9.97 | 71.75 | 99.47 |
| | l-GAN(CD) | 4.59 | 2.46 | 8.91 | 41.39 | 25.68 | 64.43 | 85.27 |
| | l-GAN(EMD) | 2.27 | 2.61 | 7.85 | 40.79 | 41.69 | 64.73 | 65.56 |
| | PC-GAN | 3.90 | 2.75 | 8.20 | 36.50 | 38.98 | 76.03 | 78.37 |
| | PointFlow | **1.74** | **2.42** | 7.87 | **46.83** | 46.98 | **60.88** | **59.89** |
| | PointGMM (ours) | 2.88 | 7.61 | **4.13** | 44.41 | **47.92** | 79.75 | 73.97 |
| car | r-GAN | 12.8 | 1.27 | 8.74 | 15.06 | 9.38 | 97.87 | 99.86 |
| | l-GAN(CD) | 4.43 | 1.55 | 6.25 | 38.64 | 18.47 | 63.07 | 88.07 |
| | l-GAN(EMD) | 2.21 | 1.48 | 5.43 | 39.20 | 39.77 | 69.74 | 68.32 |
| | PC-GAN | 3.90 | 1.12 | 5.83 | 23.56 | 30.29 | 92.19 | 90.87 |
| | PointFlow | **0.87** | **0.91** | 5.22 | **44.03** | **46.59** | **60.65** | **62.36** |
| | PointGMM (ours) | 2.25 | 3.42 | **2.82** | 40.81 | 41.90 | 90.13 | 79.78 |
| airplane | r-GAN | 7.44 | 0.261 | 5.47 | 42.72 | 18.02 | 93.58 | 99.51 |
| | l-GAN(CD) | 4.62 | 0.239 | 4.27 | 43.21 | 21.23 | 86.30 | 97.28 |
| | l-GAN(EMD) | 2.27 | 0.269 | 3.29 | **47.90** | **50.62** | 87.65 | 85.68 |
| | PC-GAN | 3.61 | 0.287 | 3.57 | 36.46 | 40.94 | 94.35 | 92.32 |
| | PointFlow | 4.92 | **0.217** | 3.24 | 46.91 | 48.40 | **75.68** | 75.06 |
| | PointGMM (ours) | **2.44** | 3.77 | **3.15** | 47.35 | 48.52 | 83.60 | **74.95** |

Table 1: Quantitative comparisons for point cloud generation.

## References


[1] Panos Achlioptas, Olga Diamanti, Ioannis Mitliagkas, and Leonidas Guibas. Learning representations and generative models for 3d point clouds. In *International Conference on Machine Learning*, pages 40–49, 2018. 11

[2] Yang et al. Pointflow: 3d point cloud generation with continuous normalizing flows. In *ICCV*, 2019. 11

[3] Chun-Liang Li, Manzil Zaheer, Yang Zhang, Barnabas Poczos, and Ruslan Salakhutdinov. Point cloud gan. *arXiv preprint arXiv:1810.05795*, 2018. 11
